# Supplementary material for: Just read twice: closing the recall gap for recurrent language models
Source: arXiv:2407.05483 source file (2024-07-07)
Supplement: Supplementary file 1 [file mamba_sd.tex]

\subsubsection{Mamba Solving SD}
We will solve the following variant of $\sd$: $|A| \le |B|$ and $A$ comes before $B$ with the elements encoded in $\{-1,1\}^d$. We take $\stateDim:= |A|$ and initialize 
\begin{align*}
\mathbf{A}_i &:= \begin{cases}
    \mathbf{I}_{2\stateDim} &\text{if } i \le |A|\\
    \begin{bmatrix}
        \mI_{\stateDim \times \stateDim} & \bm{0}_{\stateDim \times \stateDim} \\
        \vu[i,j]\cdot \mI_{\stateDim \times \stateDim} & \bm{0}_{\stateDim \times \stateDim}
    \end{bmatrix} &\text{otherwise.}
\end{cases},\\
\mathbf{B}_i &:= \begin{cases}
    \begin{bmatrix}
        \bm{e}_i & \vline & \bm{e}_{\stateDim+i}
    \end{bmatrix}^{\top} &\text{if } i < |A| \\
    \bm{0}^{2\stateDim} &\text{if } i = |A| \\
    \begin{bmatrix}
       \bm{0}^{\stateDim} & \vline  & \bm{u}[i,j] \cdot \bm{1}^{\stateDim}
    \end{bmatrix}^{\top}
     &\text{if } i > |A|
\end{cases}
\end{align*}

Recall the update equation from Mamba for SSM:
\begin{equation}
    \bm{h}[i,j] = {\mA}_{i}\bm{h}[i-1,j] + {\mB}_i\vu[i,j].
\end{equation}
For $i \in [1 \cdots |A|]$, we store the entries from $A$ in the state $\bm{h} \in \R^{\stateDim \times d}$. That is, starting with $\bm{h}[0,j] \equiv \bm{0}^{2\stateDim}$ and assuming we have
\[
\bm{h}[i-1,j] := \begin{bmatrix}
    \bm{u}[0:i-1,j] &
    \bm{0}^{\stateDim-(i-1)} &
    \vline& 
    \bm{u}[0:i-1,j] &
    \bm{0}^{\stateDim-(i-1)}
\end{bmatrix}^{\top}
\]
we get the following
\begin{align*}
\bm{h}[i,j] &= \mathbf{I}_{2\stateDim} \bm{h}[i-1,j] + \vu[i,j] \cdot \mB_i \\
&= \begin{bmatrix}
    \bm{u}[0:i-1,j] &
    \bm{0}^{\stateDim-(i-1)} &
    \vline& 
    \bm{u}[0:i-1,j] &
    \bm{0}^{\stateDim-(i-1)}
\end{bmatrix}^{\top} + \begin{bmatrix}
        \bm{u}[i,j] \cdot \bm{e}_i & \vline & \bm{u}[i,j] \cdot \bm{e}_{\stateDim+i}
    \end{bmatrix}^{\top}\\
&= \begin{bmatrix}
    \bm{u}[0:i,j] &
    \bm{0}^{\stateDim-i} &
    \vline& 
    \bm{u}[0:i,j] &
    \bm{0}^{\stateDim-i}
\end{bmatrix}^{\top}
\end{align*}
Next, for $i = |A|$, we have a separator and we skip the update by preserving the previous state. That is, for $i = |A|$, we have
\[
\bm{h}[|A|, j] \equiv \begin{bmatrix}
    \bm{u}[0:\stateDim-1,j] &
    \vline& 
    \bm{u}[0:\stateDim-1,j] &
\end{bmatrix}^{\top}
\]
Next, for $i > |A|$, we compare with the elements of $B$. For $i = |A|+1$, we have the following update:
\begin{align*}
    \bm{h}[i,j] &= \begin{bmatrix}
        \mI_{\stateDim \times \stateDim} & \bm{0}_{\stateDim \times \stateDim} \\
        \vu[i,j]\cdot \mI_{\stateDim \times \stateDim} & \bm{0}_{\stateDim \times \stateDim}
    \end{bmatrix} \begin{bmatrix}
    \bm{u}[0:\stateDim-1,j] &
    \vline& 
    \bm{u}[0:\stateDim-1,j] &
\end{bmatrix}^{\top} + \vu[i,j] \cdot \begin{bmatrix}
        \bm{0}^{\stateDim} & \bm{u}[i,j] \cdot \bm{1}^{\stateDim}
    \end{bmatrix}^{\top} \\
&= \begin{bmatrix}
    \bm{u}[0:\stateDim-1,j] &
    \vline& 
    \bm{u}[i,j] \cdot \bm{u}[0:\stateDim-1,j] &
\end{bmatrix}^{\top} + \begin{bmatrix}
                \bm{0}^{\stateDim} & \bm{1}^{\stateDim}
    \end{bmatrix}^{\top}\\
&= \begin{bmatrix}
    \bm{u}[0:\stateDim-1,j] &
    \vline& 
    \bm{u}[i,j] \cdot \bm{u}[0:\stateDim-1,j] + \bm{1}^{\stateDim}
\end{bmatrix}^{\top}
\end{align*}
Here, for $k \in [0:\stateDim-1]$, we have
\[
\bm{h}[i,j][\stateDim + k] \equiv \paren{\bm{u}[i,j] \cdot \bm{u}[0:\stateDim-1,j] + \bm{1}^{\stateDim}}[k] := \begin{cases}
    2 &\text{if }\bm{u}[i,j] = \bm{u}[k,j] \\
    0 & \text{otherwise.}
\end{cases}
\]
