# Supplementary material for: Just read twice: closing the recall gap for recurrent language models
Source: arXiv:2407.05483 source file (2024-07-07)
Supplement: Supplementary file 2 [file efficiency.tex]

\begin{table*}[h!]
    \centering
    \caption{Wall-clock time in ms by batch size for {\arch} at sequence length $16384$.}
    \label{tab:gpu_inference_jrt}
    \begin{tabular}{@{}rcccccc@{}}
    \toprule
    \textbf{Implementation}  & \textbf{2}  & \textbf{4}  & \textbf{8}  & \textbf{16} &  \textbf{32}  & \textbf{64}  \\ \midrule
    Based PyTorch        & 140.9 &  281.5  &  OOM &   OOM  &  OOM  &  OOM \\
    Based Triton (FLA)   &  4.6 &  8.7  & 16.7  &   32.4  &  64.2 & 127.8   \\
    Based Custom CUDA    &  1.2 &  1.3 & 1.5 & 2.3 & 4.5 & 8.9 \\
    \hline
    FlashAttention-2     & 3.5  &  6.7  & 13.4  &  26.6   &  52.9 & 108.2   \\
    Fast Transformer CUDA  & 17.1 &  26.7  &  50.7 &  95.5   &  OOM & OOM   \\
      \midrule
       {\arch} PyTorch   & 169.6 &  340.3  &  OOM &  OOM   &    OOM & OOM \\
       {\prompt} Custom CUDA & 2.3 &  2.5  & 2.9  &  4.5   &  9.0 & 17.8   \\
       {\arch} Custom CUDA   & 1.5  &   1.5 &  1.8 &   2.8  &  5.6 & 11.1   \\
    \bottomrule \\
    \end{tabular}
\end{table*}
